# Supplementary material for: HoloDiffusion: Training a 3D Diffusion Model using 2D Images
Source: arXiv:2303.16509 source file (2023-05-21)
Supplement: Supplementary file 1 [file holodiff_suppl.tex]

\documentclass[10pt,twocolumn,letterpaper]{article}
\usepackage{cvpr}
\usepackage{graphicx}
\usepackage{amsmath}
\usepackage{amssymb}
\usepackage{booktabs}
\usepackage{xspace}
\usepackage{todonotes}
\usepackage[pagebackref,breaklinks,colorlinks]{hyperref}
\usepackage{cleveref}
\usepackage{multirow}
\usepackage{minted}
\usepackage{cuted}

\crefname{section}{Sec.}{Secs.}
\Crefname{section}{Section}{Sections}
\Crefname{table}{Table}{Tables}
\crefname{table}{Tab.}{Tabs.}

\makeatletter
\renewcommand{\paragraph}{%
  \@startsection{paragraph}{4}%
  {\z@}{0.25em}{-1em}%
  {\normalfont\normalsize\bfseries}}
\makeatother

\input{macros}

\begin{document}

\input{suppl_body.tex}

{\small\bibliographystyle{ieee_fullname}\bibliography{holodiff,vedaldi_general,co3d_bib}}
\end{document}
